# Supplementary material for: Explaining Image Classifiers Using Contrastive Counterfactuals in Generative Latent Spaces
Source: arXiv:2206.05257 source file (2022-06-10)
Supplement: Supplementary file 1 [file 9_appendix.tex]

\clearpage
\section*{Appendix}

\subsection*{Using Contexts For Subgroup Level behavior}
We can obtain sufficiency and necessity scores from our framework for any arbitrary choice of sub-population through contexts. The context $c$ allows us to see the impact of features in specific subgroups. Using PCMs, one can express  counterfactual queries of the form $P(Y_{ A \leftarrow a}=\hat{y} \mid c)$, or simply $P(\hat{y}_{ A \leftarrow a} \mid c)$; this reads as ``For conditions  with attributes $ c$, what is the probability that we would observe $Y=\hat{y}$ had $A$ been $a$?" and is given by the following expression: 
\begin{equation}
    \begin{aligned} 
      P(\hat{y}_{ A \leftarrow a} \mid  c)
      = \sum_{z } \ P(\hat{y}_{ A \leftarrow  a}(z)) \ P( z \mid c) 
      \label{eq:context}
    \end{aligned} 
\end{equation}
 \begin{equation}
   NEC_a^{\hat{a}}(c) = P(\hat{y} _{A\leftarrow \hat{a}}|a,y,c)
  \label{eq:Nec_context}
\end{equation}
 \begin{equation}
   SUF_a^{\hat{a}}(c) = P(y _{A\leftarrow a}|\hat{a},\hat{y},c)
  \label{eq:SUF_context}
\end{equation}

For instance, we can define a context using any sensitive attribute of interest. We can obtain the scores for the target label for this sub-population of data points, and compare these scores with the general population (with an empty context) to understand different roles of features in these sub-populations. In our experiment, we obtain sufficiency and necessity scores for multiple sub-groups by setting certain attributes as the contexts. We compare these scores to the scores when the context is empty, and represents behavior on the general population. 
\begin{figure}[t]
\centering
\includegraphics[width=.7\columnwidth]{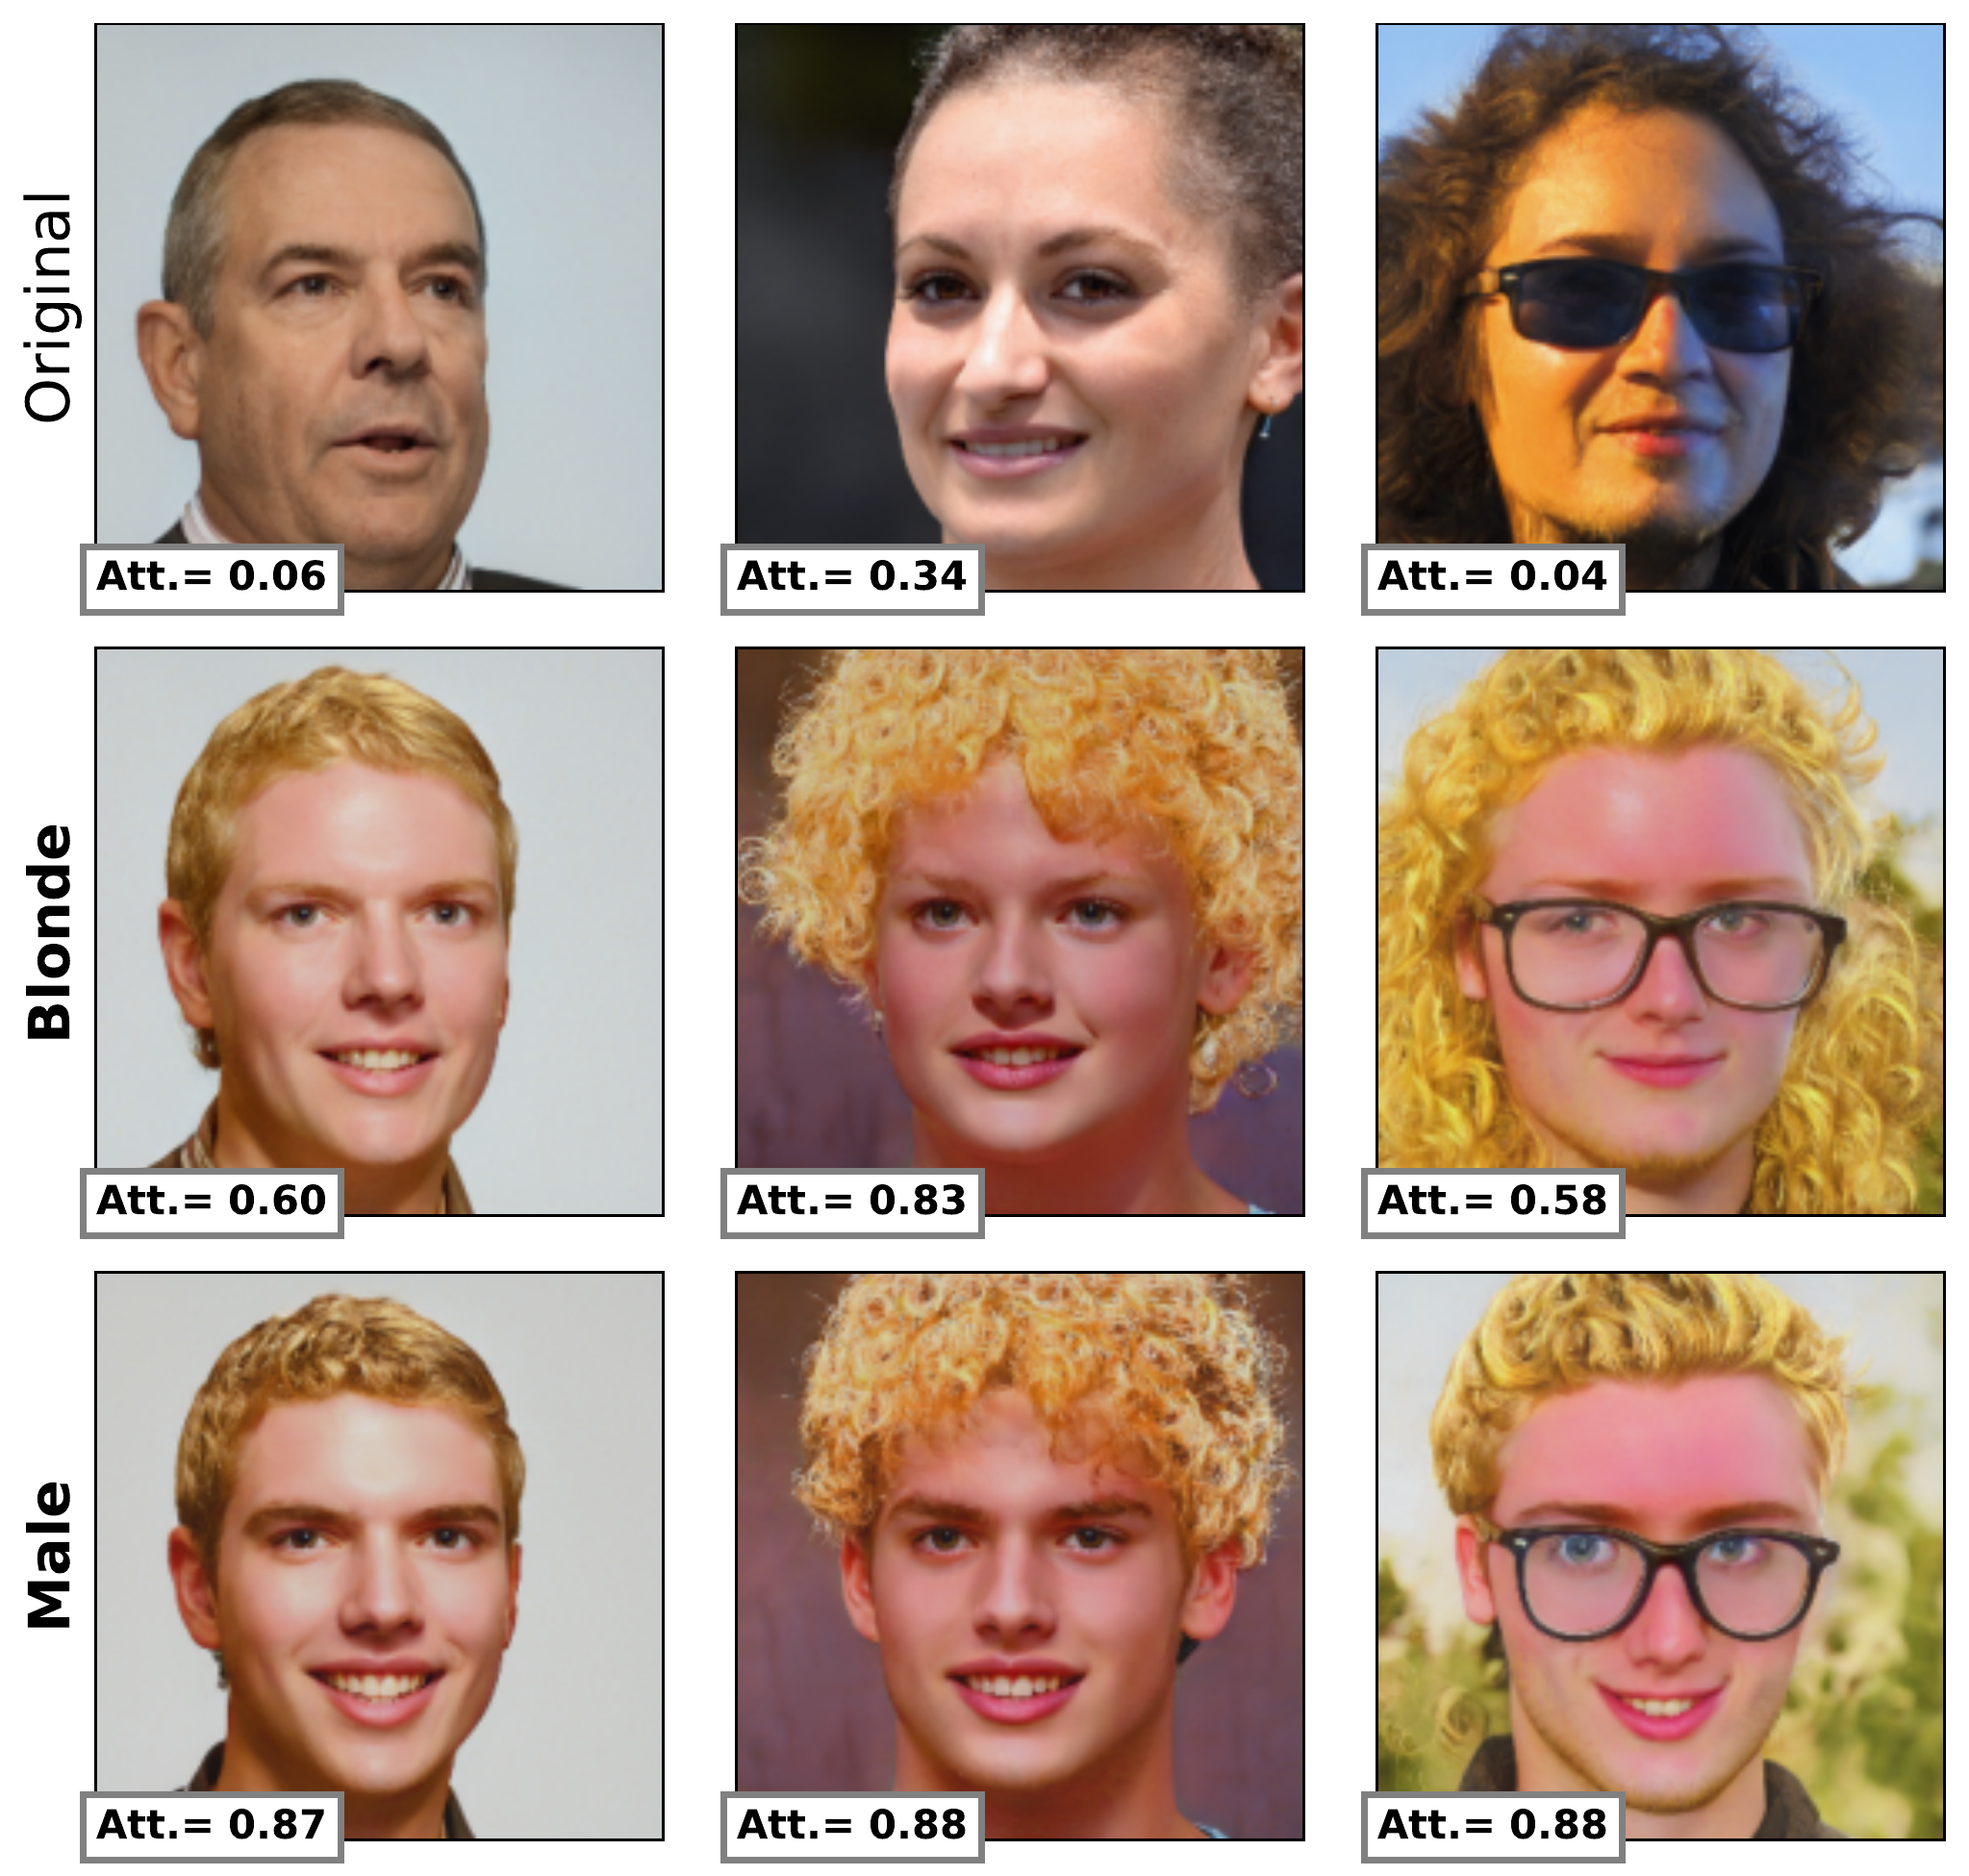}
\caption{Counterfactual image generation for computing contextual sufficiency and necessity scores. The context here is setting the attribute blond hair and we are computing scores for the attribute maleness. The attractiveness scores are at the lower left corner of each image. The original images are in the first row, followed by the counterfactual image had the context been set to high blondness. Finally, we generate the counterfactual image that has the attribute maleness set in this context.}
\label{fig:contextual_samples}
\end{figure}

Fig. \ref{fig:contextual_samples} shows how these contexts affect our scores. In this case, we are examining the effect that setting the attribute of maleness has on people who already have the blond hair attribute set. To do this, the original image is first shifted in the direction of blond hair. After this, we set the maleness attribute and see the effect that increasing maleness has on attractiveness by computing sufficiency and necessity of this shift on people with blonde hair. Of particular interest here is that our pipeline allows us to easily generate these counterfactual images with specified contexts. This enables us to produce explanations scores corresponding to any sub-group of interest. This can have multiple downstream applications, especially in group level bias analysis and mitigation. 
\todo{add graph of results of this comparison}
